# Supplementary material for: Two-Time Quantum Fluctuations Approach and its Relation to the Bethe--Salpeter Equation
Source: arXiv:2312.15034 source file (2024-02-07)
Supplement: Supplementary file 6 [file test5.tex]

%% test5.tex
%%
%% This is file `test5.tex', one of a set of several test/example files
%% in the `subfig' package.
%%
%% Copyright © 2003, 2004, 2005 Steven Douglas Cochran.
%% 
%% This work (the subfig package) may be distributed and/or modified 
%% under the conditions of the LaTeX Project Public License, either 
%% version 1.3 of this license or (at your option) any later version.
%% The latest version of this license is in
%%   http://www.latex-project.org/lppl.txt
%% and version 1.3 or later is part of all distributions of LaTeX
%% version 2003/12/01 or later.
%%
%% This work has the LPPL maintenance status "author-maintained".
%% 
%% This Current Maintainer of this work is Steven Douglas Cochran.
%%
%% This work consists of all files listed under "MANIFEST" in the
%% README file distributed with the subfig package.

\documentclass{article}

%\usepackage{captcont}
%\usepackage{caption}
%\usepackage{ccaption}

\usepackage{subfig}
\captionsetup[table]{position=top}
\captionsetup[subtable]{position=top}

%\usepackage{captcont}
%\usepackage{caption}
%\usepackage{ccaption}

\makeatletter
  \renewcommand\abstract[1]{%
    \def\@abstract{%
      \centerline{{\large\bf Abstract}}
      \noindent
      #1}}
  \renewcommand\@maketitle{%
    \newpage
    \null\vfil
    \vskip 60\p@
    \begin{center}%
      {\LARGE \@title \par}%
      \vskip 3em%
      {\large
       \lineskip .75em%
       \begin{tabular}[t]{c}%
         \@author
       \end{tabular}\par}%
      \vskip 1.5em%
      {\large \@date \par}% 
    \end{center}%
    \vskip 2.5em%
    \@abstract
    \vfil\null}%
\makeatother

\newcommand{\figbox}[2][.8in]{%
  \fbox{%
    \vbox to .6in{%
    \vfil
    \hbox to #1{%
      \hfil
      #2%
      \hfil}%
    \vfil}}}

\begin{document}

\title{Subfig Package Test Program Five}
\author{Steven Douglas Cochran\\
        Digital Mapping Laboratory\\
        School of Computer Science\\
        Carnegie-Mellon University\\
        5000 Forbes Avenue\\
        Pittsburgh, PA 15213-3890\\
        USA}
\date{21 December 2003}
\abstract{%
This test checks two things:
\begin{enumerate}
  \item the use of the references within a subfloat; and,
  \item continued floats and subfloats.
\end{enumerate}}
\maketitle
\clearpage

\setcounter{lofdepth}{2}
\listoffigures
\clearpage

\setcounter{lotdepth}{2}
\listoftables
\clearpage

In this test, we verify the ability of the subfigure package to 
handle requests for continued figures and tables (with full support
of the List-of pages and subfigures in continued figures and 
subtables in continued tables).

In addition, by varying the various included packages at the top of
the source, one can check the interaction of the subfigure package 
along with other common packages, such as the \texttt{captcont}, 
\texttt{caption}, and \texttt{ccaption} packages.

First we test the regular figures.  The first figure is
Figure~\ref{fig:First} on page \pageref{fig:First}. The second is
Figure~\ref{fig:SecondA} and appears on pages~\pageref{fig:SecondA},
\pageref{fig:SecondB}, \pageref{fig:SecondC}, and \pageref{fig:SecondD}.

\begin{figure}%
  \centering
  \figbox[4in]{Regular figure \ref{fig:First}}%
  \caption{Regular figure 1}%
  \label{fig:First}%
\end{figure}

\begin{figure}%
  \centering
  \figbox[4in]{Continued figure \ref{fig:SecondA}A}%
  \caption{Continued figure \ref{fig:SecondA}}%
  \label{fig:SecondA}%
\end{figure}

\begin{figure}%
  \ContinuedFloat
  \centering
  \figbox[4in]{Continued figure \ref{fig:SecondB}B}%
  \caption[]{Continued figure \ref{fig:SecondB}}%
  \label{fig:SecondB}%
\end{figure}

\begin{figure}%
  \ContinuedFloat
  \centering
  \figbox[4in]{Continued figure \ref{fig:SecondC}C}%
  \caption[]{Continued figure \ref{fig:SecondC}}%
  \label{fig:SecondC}%
\end{figure}

\begin{figure}%
  \ContinuedFloat
  \centering
  \figbox[4in]{Continued figure \ref{fig:SecondD}D}%
  \caption[]{Continued figure \ref{fig:SecondD}}%
  \label{fig:SecondD}%
\end{figure}

Then we test the regular tables.  The first table is
Table~\ref{tab:First} on page \pageref{tab:First}. The second is
Table~\ref{tab:SecondA} and appears on pages~\pageref{tab:SecondA},
\pageref{tab:SecondB}, \pageref{tab:SecondC}, and \pageref{tab:SecondD}.

\begin{table}%
  \centering
  \caption{Regular table 1}%
  \label{tab:First}%
  \figbox[4in]{Regular table 1}%
\end{table}

\begin{table}%
  \centering
  \caption{Continued table \ref{tab:SecondA}}%
  \label{tab:SecondA}%
  \figbox[4in]{Continued table \ref{tab:SecondA}A}%
\end{table}

\begin{table}%
  \ContinuedFloat
  \centering
  \caption[]{Continued table \ref{tab:SecondB}}%
  \label{tab:SecondB}%
  \figbox[4in]{Continued table \ref{tab:SecondB}B}%
\end{table}

\begin{table}%
  \ContinuedFloat
  \centering
  \caption[]{Continued table \ref{tab:SecondC}}%
  \label{tab:SecondC}%
  \figbox[4in]{Continued table \ref{tab:SecondC}C}%
\end{table}

\begin{table}%
  \ContinuedFloat
  \centering
  \caption[]{Continued table \ref{tab:SecondD}}%
  \label{tab:SecondD}%
  \figbox[4in]{Continued table \ref{tab:SecondD}D}%
\end{table}

Next we look at the subfloats in a simple figure.  They are
Figures~\ref{fig:sub1A}, \ref{fig:sub1B}, \ref{fig:sub1C}, and
\ref{fig:sub1D}, which are part of Figure~\ref{fig:sub1} on 
page~\pageref{fig:sub1}.

The continued subfloats are contained in three parts.  The first is
Figure~\ref{fig:sub21} on page~\pageref{fig:sub21} which contains the
Subfigures~\ref{fig:sub2A}, \ref{fig:sub2B}, \ref{fig:sub2C}, and
\ref{fig:sub2D}.
The second is
Figure~\ref{fig:sub22} on page~\pageref{fig:sub22} which contains the
Subfigures~\ref{fig:sub2E}, \ref{fig:sub2F}, \ref{fig:sub2G}, and
\ref{fig:sub2H}.
The third is
Figure~\ref{fig:sub23} on page~\pageref{fig:sub23} which contains the
Subfigures~\ref{fig:sub2I}, \ref{fig:sub2J}, \ref{fig:sub2K}, and
\ref{fig:sub2L}.

\begin{figure}%
  \centering
  \subfloat[\label{fig:sub1A}]{\figbox{Subfigure \ref{fig:sub1A}}}
  \hspace{10pt}%
  \subfloat[\label{fig:sub1B}]{\figbox{Subfigure \ref{fig:sub1B}}} \\
  \subfloat[\label{fig:sub1C}]{\figbox{Subfigure \ref{fig:sub1C}}}
  \hspace{10pt}%
  \subfloat[\label{fig:sub1D}]{\figbox{Subfigure \ref{fig:sub1D}}}
  \caption{This is a simple figure.}%
  \label{fig:sub1}%
\end{figure}

\begin{figure}%
  \centering
  \subfloat[\label{fig:sub2A}]{\figbox{Subfigure \ref{fig:sub2A}}}
  \hspace{10pt}%
  \subfloat[\label{fig:sub2B}]{\figbox{Subfigure \ref{fig:sub2B}}} \\
  \subfloat[\label{fig:sub2C}]{\figbox{Subfigure \ref{fig:sub2C}}}
  \hspace{10pt}%
  \subfloat[\label{fig:sub2D}]{\figbox{Subfigure \ref{fig:sub2D}}}
  \caption{This is a continued figure.}%
  \label{fig:sub21}%
\end{figure}
  
\begin{figure}%
  \ContinuedFloat
  \centering
  \subfloat[\label{fig:sub2E}]{\figbox{Subfigure \ref{fig:sub2E}}}
  \hspace{10pt}%
  \subfloat[\label{fig:sub2F}]{\figbox{Subfigure \ref{fig:sub2F}}} \\
  \subfloat[\label{fig:sub2G}]{\figbox{Subfigure \ref{fig:sub2G}}}
  \hspace{10pt}%
  \subfloat[\label{fig:sub2H}]{\figbox{Subfigure \ref{fig:sub2H}}}
  \caption[]{This is a continued figure (cont.)}%
  \label{fig:sub22}%
\end{figure}

\begin{figure}%
  \ContinuedFloat
  \centering
  \subfloat[\label{fig:sub2I}]{\figbox{Subfigure \ref{fig:sub2I}}}
  \hspace{10pt}%
  \subfloat[\label{fig:sub2J}]{\figbox{Subfigure \ref{fig:sub2J}}} \\
  \subfloat[\label{fig:sub2K}]{\figbox{Subfigure \ref{fig:sub2K}}}
  \hspace{10pt}%
  \subfloat[\label{fig:sub2L}]{\figbox{Subfigure \ref{fig:sub2L}}}
  \caption[]{This is a continued figure (cont.)}%
  \label{fig:sub23}%
\end{figure}

Next we look at the subfloats in a simple table environment.  They are
Tables~\ref{tab:sub1A}, \ref{tab:sub1B}, \ref{tab:sub1C}, and
\ref{tab:sub1D}, which are part of Table~\ref{tab:sub1} on 
page~\pageref{tab:sub1}.

The continued subfloats are contained in three parts.  The first is
Table~\ref{tab:sub21} on page~\pageref{tab:sub21} which contains the
Subtables~\ref{tab:sub2A}, \ref{tab:sub2B}, \ref{tab:sub2C}, and
\ref{tab:sub2D}.
The second is
Table~\ref{tab:sub22} on page~\pageref{tab:sub22} which contains the
Subtables~\ref{tab:sub2E}, \ref{tab:sub2F}, \ref{tab:sub2G}, and
\ref{tab:sub2H}.
The third is
Table~\ref{tab:sub23} on page~\pageref{tab:sub23} which contains the
Subtables~\ref{tab:sub2I}, \ref{tab:sub2J}, \ref{tab:sub2K}, and
\ref{tab:sub2L}.

\begin{table}%
  \centering
  \caption{This is a simple table.}%
  \label{tab:sub1}%
  \subfloat[\label{tab:sub1A}]{\figbox{Subtable \ref{tab:sub1A}}}
  \hspace{10pt}%
  \subfloat[\label{tab:sub1B}]{\figbox{Subtable \ref{tab:sub1B}}} \\
  \subfloat[\label{tab:sub1C}]{\figbox{Subtable \ref{tab:sub1C}}}
  \hspace{10pt}%
  \subfloat[\label{tab:sub1D}]{\figbox{Subtable \ref{tab:sub1D}}}
\end{table}

\begin{table}%
  \centering
  \caption{This is a continued table.}%
  \label{tab:sub21}%
  \subfloat[\label{tab:sub2A}]{\figbox{Subtable \ref{tab:sub2A}}}
  \hspace{10pt}%
  \subfloat[\label{tab:sub2B}]{\figbox{Subtable \ref{tab:sub2B}}} \\
  \subfloat[\label{tab:sub2C}]{\figbox{Subtable \ref{tab:sub2C}}}
  \hspace{10pt}%
  \subfloat[\label{tab:sub2D}]{\figbox{Subtable \ref{tab:sub2D}}}
\end{table}

\begin{table}%
  \ContinuedFloat
  \centering
  \caption[]{This is a continued table (cont.)}%
  \label{tab:sub22}%
  \subfloat[\label{tab:sub2E}]{\figbox{Subtable \ref{tab:sub2E}}}
  \hspace{10pt}%
  \subfloat[\label{tab:sub2F}]{\figbox{Subtable \ref{tab:sub2F}}} \\
  \subfloat[\label{tab:sub2G}]{\figbox{Subtable \ref{tab:sub2G}}}
  \hspace{10pt}%
  \subfloat[\label{tab:sub2H}]{\figbox{Subtable \ref{tab:sub2H}}}
\end{table}

\begin{table}%
  \ContinuedFloat
  \centering
  \caption[]{This is a continued table (cont.)}%
  \label{tab:sub23}%
  \subfloat[\label{tab:sub2I}]{\figbox{Subtable \ref{tab:sub2I}}}
  \hspace{10pt}%
  \subfloat[\label{tab:sub2J}]{\figbox{Subtable \ref{tab:sub2J}}} \\
  \subfloat[\label{tab:sub2K}]{\figbox{Subtable \ref{tab:sub2K}}}
  \hspace{10pt}%
  \subfloat[\label{tab:sub2L}]{\figbox{Subtable \ref{tab:sub2L}}}
\end{table}

\end{document}
