# Supplementary material for: Two-Time Quantum Fluctuations Approach and its Relation to the Bethe--Salpeter Equation
Source: arXiv:2312.15034 source file (2024-02-07)
Supplement: Supplementary file 8 [file test7.tex]

%% test7.tex
%%
%% This is file `test7.tex', one of a set of several test/example files
%% in the `subfig' package.
%%
%% Copyright © 2003, 2004, 2005 Steven Douglas Cochran.
%% 
%% This work (the subfig package) may be distributed and/or modified 
%% under the conditions of the LaTeX Project Public License, either 
%% version 1.3 of this license or (at your option) any later version.
%% The latest version of this license is in
%%   http://www.latex-project.org/lppl.txt
%% and version 1.3 or later is part of all distributions of LaTeX
%% version 2003/12/01 or later.
%%
%% This work has the LPPL maintenance status "author-maintained".
%% 
%% This Current Maintainer of this work is Steven Douglas Cochran.
%%
%% This work consists of all files listed under "MANIFEST" in the
%% README file distributed with the subfig package.

\documentclass{article}

\makeatletter
%% We pretend that we are a naughty class and are \let'ting our
%% \endfigure to the \end@float, etc.

\def\thefigure{\@arabic\c@figure}
\def\fps@figure{tbp}
\def\ftype@figure{1}
\def\ext@figure{lof}
\def\fnum@figure{Fig.~\thefigure}
\def\figure{\@float{figure}}
%% This is the bad line, it should be "\def\endfigure{\end@float}"
\let\endfigure\end@float
\@namedef{figure*}{\@dblfloat{figure}}
\@namedef{endfigure*}{\end@dblfloat}

\def\thetable{\@Roman\c@table}
\def\fps@table{tbp}
\def\ftype@table{2}
\def\ext@table{lot}
\def\fnum@table{TABLE~\thetable}
\def\table{%
  \def\@floatboxreset{\reset@font\footnotesize\@setminipage}%
  \@float{table}}
%% This is the bad line, it should be "\def\endtable{\end@float}"
\let\endtable\end@float
\@namedef{table*}{%
  \def\@floatboxreset{\reset@font\footnotesize\@setminipage}%
  \@dblfloat{table}}
\@namedef{endtable*}{\end@dblfloat}
\makeatother

% Next we load the subfig package and see if it finds the problem.
% To check this test result, you need to see the TTY listing or check
% the test5.log (which we save as test5b.ps).
\usepackage[position=top,nearskip=10pt,lofdepth,lotdepth]{subfig}

\newcommand{\figbox}[1]{%
  \fbox{%
    \vbox to 1in{%
    \vfil
    \hbox to 2in{%
      \hfil
      {\normalsize #1}%
      \hfil}%
    \vfil}}}

\newcommand{\goodgap}{\hspace{9pt}}

\begin{document}
\listoffigures
\listoftables
\newpage

\section{Seventh Test}

\begin{figure}%
  \centering
  \caption{Figure One.}%
  \label{fig:first}%
  \subfloat[Figure subone.\label{fig:first:A}]{\figbox{Figure subone}}%
  \goodgap
  \subfloat[Figure subtwo.\label{fig:first:B}]{\figbox{Figure subtwo}}\\
  \subfloat[Figure subthree.\label{fig:first:C}]{\figbox{Figure subthree}}%
  \goodgap
  \subfloat[Figure subfour.\label{fig:first:D}]{\figbox{Figure subfour}}%
\end{figure}

\begin{figure}%
  \ContinuedFloat
  \centering
  \caption[]{Figure One (cont.)}%
  \label{fig:first_cont}%
  \subfloat[Figure subfive.\label{fig:first:E}]{\figbox{Figure subfive}}
  \goodgap
  \subfloat[Figure subsix.\label{fig:first:F}]{\figbox{Figure subsix}} \\
  \subfloat[Figure subseven.\label{fig:first:G}]{\figbox{Figure subseven}}
  \goodgap
  \subfloat[Figure subeight.\label{fig:first:H}]{\figbox{Figure subeight}}
\end{figure}

This test checks to see if the subfig package reacts correctly to the
known sort of problem class.  We check that on the list-of-figures page
the continued figure correctly labeled from (a) to (h) and that on the
list-of-tables page, the table has the two subcaptions in addition to the
main caption.  If not, than the nasty class has zapped us.

(We also need to check the test7.log file to insure that the problem
was identified by the subfig package and a warning was issued.)

\begin{table}[t]%
  \centering
  \caption{Table One.}%
  \label{tab:first}%
  \subfloat[Table subone.\label{tab:first:A}]{\figbox{Table subone}}  \goodgap
  \subfloat[Table subtwo.\label{tab:first:B}]{\figbox{Table subtwo}}%
\end{table}

\end{document}
